# Supplementary material for: Revisiting Hotels-50K and Hotel-ID
Source: arXiv:2207.10200 source file (2022-07-20)
Supplement: Supplementary file 1 [file a020imagelinking.tex]

\begin{figure*}
    \centering
    \includegraphics[width=.9\textwidth]{imgs/fig1_pdf.pdf}
    \caption{Images from the same hotel may (left) or may not (right) be connected, while images from different hotels may be connected (middle). Here, we have example images from four different hotels. Images from the same hotel are indicated with the same border color. We see that not all of the images in the same class are connected to each other (only purple class has all the pairwise connections between the examples). We also see that different classes can be connected to each other due to similar features (e.g., red and green class which share the same carpet).}
    \label{fig:image-linking}
\end{figure*}
\section{Image Linking}
\label{sec:imagelinking}

% Draw connection with link prediction in graphs
% Image retrieval has labels on nodes
We define ``image linking'' as a subset of deep metric learning (DML) methods with the objective of connecting pairs of images based on their commonalities and connecting images \textit{only} if they share a common feature. This task requires the trained model to extract a single (or multiple) feature vectors for each image and focus on the shared features of every given pair. 
% Although this task is a subset of DML and it may be argued that the representations learned in image retrieval or classification can be used for this purpose, however, the objectives of these ;
Due to the subtle difference between image linking and image classification (or retrieval), the representations learned in the latter tasks may not be optimal for image linking.
More specifically, given a dataset of size $N$ with $M$ different classes, as opposed to image classification (retrieval) that for every image $img_i$ a label $l_i \in L$ is assigned where $L = \{1, 2, ..., M\}$, image linking defines a matrix $Y = \{0, 1\}^{N \times N}$, which assigns a label $Y_{ij}$ for pairs of images $img_i$ and $img_j$, depending on whether they share a feature. The matrix $Y$ represents which pairs of images in the dataset have features in common. An analogy between image classification and image linking is the distinction between \textit{node} and \textit{link} classification in graphs, in which $Y$ would be the adjacency matrix. Considering this distinction, we suggest using metrics mostly common in link prediction, e.g. area under the receiver operating curve (AUROC), rather than the more commonly used metrics in DML, e.g. Recall@K, aiming to reduce the incorrect connections as much as possible. Figure \ref{fig:image-linking} provides an illustration for this task where classes defined as hotel rooms do not correspond exactly to links between pairs of images, which can for example indicate the rooms sharing a same carpet or curtain. 

To evaluate this task with AUROC, we sample an equal number of positive and negative image pairs in order for the model to predict their connections. In this study, we \textit{randomly} sample a negative and positive sample per each evaluation image to avoid additional computation cost (we refer to this metric as \randauroc). Nevertheless, due to the large pool of negative images for any given image, the chosen negative sample can be extremely different from the image and hence, easy to predict their irrelevance. As such, we consider a second evaluation setting in which we carefully construct a set of negative images for each image in the dataset using a pre-trained ResNet50 (before being fine-tuned on these datasets). In particular, to create the set of hard negatives, we use a pre-trained ResNet50 on ImageNet to extract the image embeddings and mine the most similar negative images for each sample (referred to as \newauroc).
